# Supplementary material for: Face Recognition Accuracy Across Demographics: Shining a Light Into the Problem
Source: arXiv:2206.01881 source file (2023-04-16)
Supplement: Supplementary file 1 [file supplementary_marterial_figures.tex]

\begin{figure}[h]
    \centering
    \begin{subfigure}[b]{1\linewidth}
    \captionsetup[subfigure]{labelformat=empty}
        \begin{subfigure}[b]{1\linewidth}
            \begin{subfigure}[b]{1\linewidth}
            \centering
                \begin{subfigure}[b]{0.15\linewidth}
                    \includegraphics[width=\linewidth]{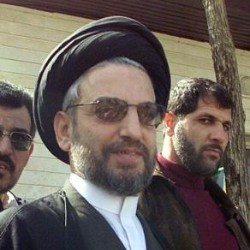}
                    
                \end{subfigure}
                \begin{subfigure}[b]{0.15\linewidth}
                    \includegraphics[width=\linewidth]{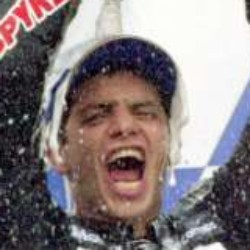}
                    
                \end{subfigure}
                \begin{subfigure}[b]{0.15\linewidth}
                    \includegraphics[width=\linewidth]{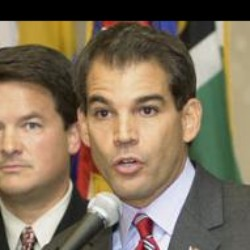}
                    
                \end{subfigure}
                \begin{subfigure}[b]{0.15\linewidth}
                    \includegraphics[width=\linewidth]{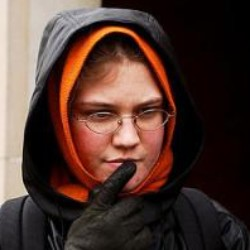}
                    
                \end{subfigure}
                \begin{subfigure}[b]{0.15\linewidth}
                    \includegraphics[width=\linewidth]{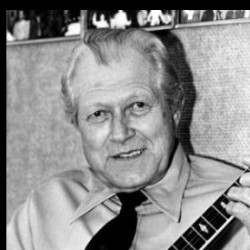}
                    
                \end{subfigure}
                \begin{subfigure}[b]{0.15\linewidth}
                    \includegraphics[width=\linewidth]{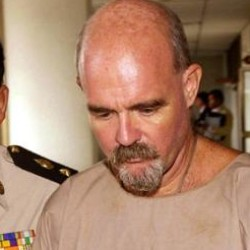}
                    
                \end{subfigure}
            \end{subfigure}
        \end{subfigure}
        \begin{subfigure}[b]{1\linewidth}
            \begin{subfigure}[b]{1\linewidth}
            \centering
                \begin{subfigure}[b]{0.15\linewidth}
                    \includegraphics[width=\linewidth]{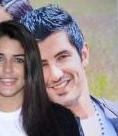}
                    
                \end{subfigure}
                \begin{subfigure}[b]{0.15\linewidth}
                    \includegraphics[width=\linewidth]{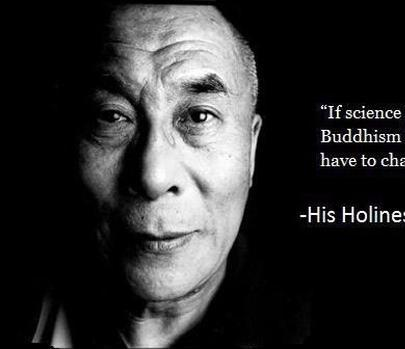}
                    
                \end{subfigure}
                \begin{subfigure}[b]{0.15\linewidth}
                    \includegraphics[width=\linewidth]{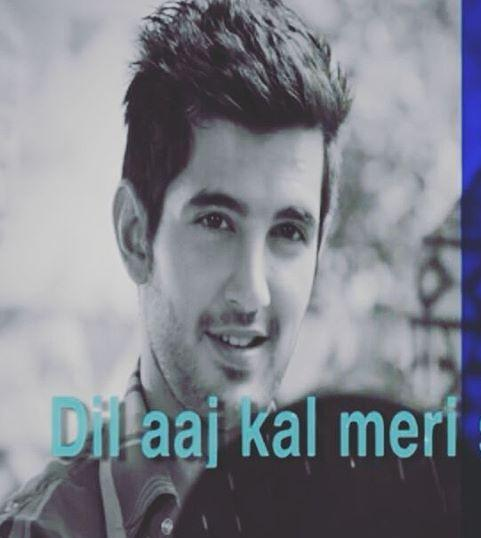}
                    
                \end{subfigure}
                \begin{subfigure}[b]{0.15\linewidth}
                    \includegraphics[width=\linewidth]{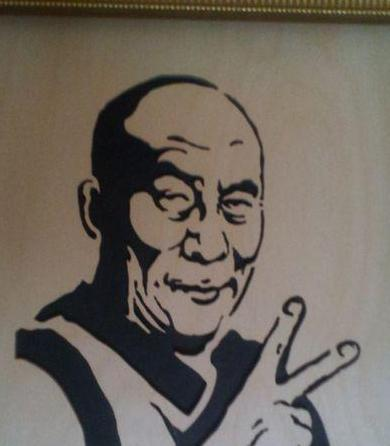}
                    
                \end{subfigure}
                \begin{subfigure}[b]{0.15\linewidth}
                    \includegraphics[width=\linewidth]{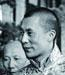}
                    
                \end{subfigure}
                \begin{subfigure}[b]{0.15\linewidth}
                    \includegraphics[width=\linewidth]{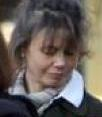}
                \end{subfigure}
            \end{subfigure}
        \end{subfigure}
        \begin{subfigure}[b]{1\linewidth}
            \begin{subfigure}[b]{1\linewidth}
            \centering
                \begin{subfigure}[b]{0.15\linewidth}
                    \includegraphics[width=\linewidth]{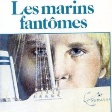}
                    
                \end{subfigure}
                \begin{subfigure}[b]{0.15\linewidth}
                    \includegraphics[width=\linewidth]{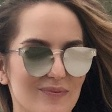}
                    
                \end{subfigure}
                \begin{subfigure}[b]{0.15\linewidth}
                    \includegraphics[width=\linewidth]{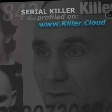}
                    
                \end{subfigure}
                \begin{subfigure}[b]{0.15\linewidth}
                    \includegraphics[width=\linewidth]{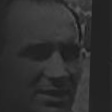}
                    
                \end{subfigure}
                \begin{subfigure}[b]{0.15\linewidth}
                    \includegraphics[width=\linewidth]{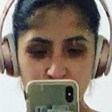}
                    
                \end{subfigure}
                \begin{subfigure}[b]{0.15\linewidth}
                    \includegraphics[width=\linewidth]{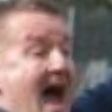}
                \end{subfigure}
            \end{subfigure}
        \end{subfigure}
    \end{subfigure}
   \caption{Samples of three widely used web-scrapped datasets. The samples in the first, second, third row are from LFW, VGGFace2, and WebFace260M respectively.}
\label{fig:web-scrapped-samples}
\end{figure}
